# Supplementary material for: State of What Art? A Call for Multi-Prompt LLM Evaluation
Source: arXiv:2401.00595 source file (2024-05-06)
Supplement: Supplementary file 1 [file 99_appendix.tex]

\remove{
\subsection{Tasks - Additional Details}
\label{sec:appendix_tasks_info}
% Please add the following required packages to your document preamble:
% \usepackage{booktabs}
% \usepackage{multirow}
% \usepackage{graphicx}
\begin{table*}[bt!]
\begin{adjustwidth}{-1cm}{-1cm}
\small
\centering
% \resizebox{\textwidth}{!}{
\begin{tabular}{lp{11cm}}
\toprule
Benchmark \& Task & Instruction Template \\ \midrule
\textbf{\lmentry{}} \\
$\quad$ all words from category & Q: Are all the words \{$words$\} types of \{$category$\}? Answer either ``yes'' or ``no''.
A:\\
 $\quad$ any words from category & Q: Does the list [\{$words$\}] contain any \{$category$\}? Answer either ``yes'' or ``no''.
A: \\
$\quad$ ends with word & Write a sentence that ends with the word ``\{$word$\}'': \\
$\quad$ first alphabetically & Q: In an alphabetical order, which word comes first, ``\{$word1$\}'' or ``\{$word2$\}''?
A: \\
$\quad$ homophones & Q: Which word sounds like the word ``\{$query$\}'', ``\{$word1$\}'' or ``\{$word2$\}''?
A: \\
$\quad$ less letters & Q: Which word is shorter, ``\{$word1$\}'' or ``\{$word2$\}''?
A: \\
$\quad$ more letters & Q: Which word has more letters, ``\{$word1$\}'' or ``\{$word2$\}''?
A: \\
$\quad$ rhyming word & Q: Which is a rhyme of the word ``\{$query$\}'', ``\{$word1$\}'' or ``\{$word2$\}''?
 A: \\
$\quad$ word before & Q: Which word comes right before ``\{$word$\}'' in the sentence ``\{$sentence$\}''?
A: \\
$\quad$ word not containing & Write a word that doesn't contain the letter ``\{$letter$\}'':
  \\\midrule

\textbf{\bigbenchlite{}}\\
$\quad$ bbq lite    &    \{$input$\}
option: \{$option1$\}
option: \{$option2$\}
option: \{$option3$\}
Answer: 
         \\
$\quad$    code line description    &  Python code:
\{$input$\}
choice: \{$option1$\}
choice: \{$option2$\}
choice: \{$option3$\}
choice: \{$option4$\}

English language description:           \\
$\quad$   conceptual combinations     &    \{$input$\}
option: \{$option1$\}
option: \{$option2$\}
option: \{$option3$\}
option: \{$option4$\}
Answer:          \\
$\quad$    hindu knowledge    &     Q: \{$input$\}
choice: \{$option1$\}
choice: \{$option2$\}
choice: \{$option3$\}
choice: \{$option4$\}
A:         \\
$\quad$   known unknown    &    \{$input$\}
choice: \{$option1$\}
choice: \{$option2$\}
          \\
$\quad$    language identification    &   Given a sentence, select the correct language among the choices
Sentence: \{$input$\}
choice: \{$option1$\}
choice: \{$option2$\}
choice: \{$option3$\}
choice: \{$option4$\}
...
Language:          \\
$\quad$     logic grid puzzle   &    \{$input$\}
                                  Answer:\\
$\quad$    logical deduction   &  The following paragraphs each describe a set of three objects arranged in a fixed order. The statements are logically consistent within each paragraph.

\{$input$\} 
           \\
$\quad$    novel concepts    &   Let's do some find-the-common-concept problems. In these problems, your goal is to identify the underlying concept or theme that relates the things listed. Make sure to answer carefully.
\{$input$\}
Answer:
          \\
$\quad$    play dialog    & The following transcripts of dialogues have been taken from Shakespeare plays, but the transcripts do not say who said what.  Your task is to identify whether the sentences in question were spoken by the same or different people.
Dialogue:
\{$input$\}
Answer:
           \\
$\quad$    strange stories     &   Context: \{$input$\}
choice: \{$option1$\}
choice: \{$option2$\}
choice: \{$option3$\}
choice: \{$option4$\}
A:
          \\
$\quad$    strategic qa    &   Q: \{$input$\}
A:
          \\
$\quad$    vitaminc fact verification    &  Based only on the information contained in a brief quote from Wikipedia, answer whether the related claim is True, False or Neither. Use Neither when the Wikipedia quote does not provide the necessary information to resolve the question.

Passage:
\{$input$\}

True, False, or Neither?
           \\
$\quad$     winowhy   &   Please answer the following questions about which words certain pronouns refer to.
\{$input$\}
The above reasoning is          \\ \midrule

 \textbf{\bigbenchhard{}} \\
$\quad$  causal judgement    & How would a typical person answer each of the following questions about causation? \\
% \{$question$\}
% Options:
% - Yes
% - No
% A:             \\
$\quad$ disambiguation qa    & In the following sentences, explain the antecedent of the pronoun (which thing the pronoun refers to), or state that it is ambiguous. \\
% Sentence: \{$sentence$\}
% Options:
% \{$options$\}
% A:            \\
$\quad$ formal fallacies   &  Is the argument, given the explicitly stated premises, deductively valid or invalid? \\
% Options:
% - valid
% - invalid
% A:           \\
$\quad$  geometric shapes    & This SVG path element \{$svg\_path\_element$\} draws a  Options: \{$options$\} \\
% A:            \\
$\quad$ hyperbaton   & Which sentence has the correct adjective order: \\
% Options:
% \{$options$\}
% A:            \\
$\quad$ logical deduction five objects    &  QThe following paragraphs each describe a set of five objects arranged in a fixed order. The statements are logically consistent within each paragraph. \\
% \{$paragraph$\}
% Options:
% \{$options$\}
% A:           \\
$\quad$ logical deduction seven objects    &  The following paragraphs each describe a set of seven objects arranged in a fixed order. The statements are logically consistent within each paragraph \\
% \{$paragraph$\}
% Options:
% \{$options$\}
% A:           \\
$\quad$  logical deduction three objects   &  The following paragraphs each describe a set of three objects arranged in a fixed order. The statements are logically consistent within each paragraph. \\
% \{$paragraph$\}
% Options:
% \{$options$\}
% A:           \\
$\quad$ movie recommendation    &  Find a movie similar to \{$movie\_list$\} \\
% Options:
% \{$options$\}
% A:           \\
$\quad$  navigate    & If you follow these instructions, do you return to the starting point? \\
% \{$instructions$\}
% Options:
% - Yes
% - No
% A:            \\
$\quad$  penguins in a table   & Here is a table where the first line is a header and each subsequent line is a penguin:  name, age, height (cm), weight (kg)  \{$question$\} \\
% \{$table\_description$\}
% \{$question$\}
% Options:
% \{$options$\}
% A:            \\
$\quad$  ruin names    & Q: Which of the following is a humorous edit of this artist or movie name: '\{$artist\_or\_movie\_name$\}'? \\
% Options:
% \{$options$\}
% A:
%             \\
$\quad$   salient translation error detection    &  The following translations from German to English contain a particular error. That error will be one of the following types: $\ldots$ Please identify that error. \\
% Source: \{$source$\}
% Translation: \{$translation$\}
% The translation contains an error pertaining to
% Options:
% \{$options$\}
% A:
%            \\
$\quad$  snarks    & Which statement is sarcastic? \\
% Options:
% \{$options$\}
% A:
%             \\
$\quad$  sports understanding    & Q: Is the following sentence plausible? \\
% ``\{$sentence$\}''
% A:
\\ \bottomrule

\end{tabular}%
%}
\caption{The 39 tasks used in this paper, along with the benchmarks from which they were taken and an example task instruction.}
\label{tab:tasks}
\end{adjustwidth}
\end{table*}
Table~\ref{tab:tasks} presents an overview of the 39 tasks from the 3 benchmarks discussed in this paper: \lmentry{}, \bigbenchlite{}, and \bigbenchhard{}. These benchmarks include 10, 14, and 15 tasks from each, respectively. The table also provides an example task instruction for each task.

\subsection{Process of Generating Prompt Paraphrases}
\label{sec:appendix_prompt_generation}
Our process for generating paraphrases of instruction templates is depicted with an example in Figure~\ref{fig:metaprompts}.

\begin{figure*}[p]
\includegraphics[width=\textwidth]{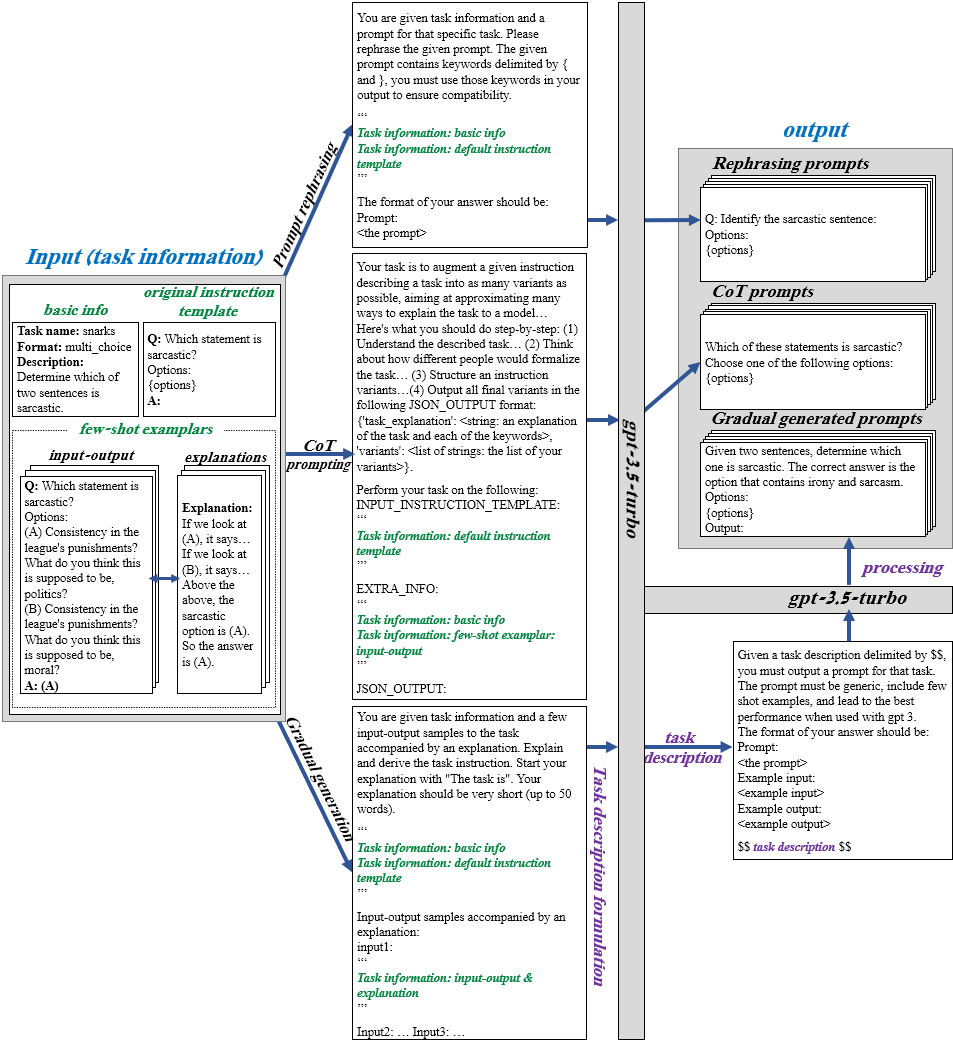}
\caption{\label{fig:metaprompts} 
Our process for automatically generating paraphrases of instruction templates, using the 'snarks' task from the BBH benchmark as an example. We input task information from the benchmark, including basic details, the original instruction template, and a few-shot exemplar, into various meta-prompts tailored to different generation methods (prompt rephrasing, CoT prompting, or gradual generation). Then, we feed these meta-prompts into \cgpt{} to create new instruction templates for the given task. Notably, in the gradual generation method, \cgpt{} is utilized twice: initially to generate a detailed task description, and subsequently to derive a new instruction template from it.}
\end{figure*}

\subsection{Paraphrases Correctness}
\label{sec:appendix_paraph_correct}
Tables~\ref{table:paraphrases_correctness_lmentry} and~\ref{table:paraphrases_correctness_bbh} present the percentages of correct paraphrases that were generated by the 3 prompt-generating methods presented in the paper for \lmentry{} and BBH. The tables also depict the average model accuracy and standard deviations as measured for only the correct paraphrases across all LLMs. The correct paraphrases were identified by one of the authors of this paper.
Table~\ref{tab:metric_rankings_comparisson} presents the Kendall $\tau$ values before and after the removal of incorrect paraphrases. The agreement in the ranking of models is near-perfect to perfect in both \lmentry{} and BBH benchmarks.
% Please add the following required packages to your document preamble:
% \usepackage{graphicx}
\begin{table*}[bt!]
\small
\resizebox{\textwidth}{!}{%
\begin{tabular}{l|lccccc}
\toprule
\textbf{Benchmark \& Task}          & \textbf{Method}                                                        & \textbf{\begin{tabular}[c]{@{}c@{}}\#Auto \\ Paraphrases\end{tabular}}                                     & \textbf{\begin{tabular}[c]{@{}c@{}}\#Correct \\ Paraphrases\end{tabular}}                                  & \textbf{\begin{tabular}[c]{@{}l@{}}Correct \\ Ratio (\%)\end{tabular}}                                                   & \textbf{\begin{tabular}[c]{@{}l@{}}Model\\ Accuracy \\ (Avg.)\end{tabular}}                                & \textbf{\begin{tabular}[c]{@{}l@{}}Model\\ Accuracy \\ (Std.)\end{tabular}}                               \\
\hline
 all words from category             & \begin{tabular}[c]{@{}l@{}}All\\ Rephrase\\ CoT\\ Gradual\end{tabular} & \begin{tabular}[c]{@{}l@{}}258\\ 48\\ 133\\ 74\end{tabular}     & \begin{tabular}[c]{@{}l@{}}227\\ 39\\ 131\\ 54\end{tabular}     & \begin{tabular}[c]{@{}l@{}}87.98\%\\ 81.25\%\\ 98.50\%\\ 72.97\%\end{tabular} & \begin{tabular}[c]{@{}l@{}}.519\\ .483\\ .494\\ .604\end{tabular}  & \begin{tabular}[c]{@{}l@{}}.074\\ .035\\ .065\\ .048\end{tabular} \\ \midrule
any words from category             & \begin{tabular}[c]{@{}l@{}}All\\ Rephrase\\ CoT\\ Gradual\end{tabular} & \begin{tabular}[c]{@{}l@{}}259\\ 48\\ 135\\ 72\end{tabular}     & \begin{tabular}[c]{@{}l@{}}233\\ 44\\ 134\\ 52\end{tabular}     & \begin{tabular}[c]{@{}l@{}}89.96\%\\ 91.67\%\\ 99.26\%\\ 71.23\%\end{tabular} & \begin{tabular}[c]{@{}l@{}}.443\\ .451\\ .438\\ .444\end{tabular}  & \begin{tabular}[c]{@{}l@{}}.083\\ .043\\ .034\\ .160\end{tabular} \\ \midrule
ends with word                      & \begin{tabular}[c]{@{}l@{}}All\\ Rephrase\\ CoT\\ Gradual\end{tabular} & \begin{tabular}[c]{@{}l@{}}226\\ 47\\ 129\\ 47\end{tabular}     & \begin{tabular}[c]{@{}l@{}}210\\ 39\\ 126\\ 42\end{tabular}     & \begin{tabular}[c]{@{}l@{}}92.92\%\\ 82.98\%\\ 97.67\%\\ 89.36\%\end{tabular} & \begin{tabular}[c]{@{}l@{}}.131\\ .130\\ .138\\ .112\end{tabular}  & \begin{tabular}[c]{@{}l@{}}.024\\ .022\\ .019\\ .027\end{tabular} \\ \midrule
first alphabetically                & \begin{tabular}[c]{@{}l@{}}All\\ Rephrase\\ CoT\\ Gradual\end{tabular} & \begin{tabular}[c]{@{}l@{}}233\\ 47\\ 121\\ 62\end{tabular}     & \begin{tabular}[c]{@{}l@{}}198\\ 38\\ 117\\ 40\end{tabular}     & \begin{tabular}[c]{@{}l@{}}84.98\%\\ 80.85\%\\ 96.69\%\\ 64.52\%\end{tabular} & \begin{tabular}[c]{@{}l@{}}.326\\ .293\\ .315\\ .381\end{tabular}  & \begin{tabular}[c]{@{}l@{}}.079\\ .080\\ .076\\ .053\end{tabular} \\ \midrule
homophones                          & \begin{tabular}[c]{@{}l@{}}All\\ Rephrase\\ CoT\\ Gradual\end{tabular} & \begin{tabular}[c]{@{}l@{}}264\\ 48\\ 140\\ 73\end{tabular}     & \begin{tabular}[c]{@{}l@{}}234\\ 43\\ 128\\ 60\end{tabular}     & \begin{tabular}[c]{@{}l@{}}88.64\%\\ 89.58\%\\ 91.43\%\\ 82.19\%\end{tabular} & \begin{tabular}[c]{@{}l@{}}.252\\ .214\\ .246\\ .292\end{tabular}  & \begin{tabular}[c]{@{}l@{}}.057\\ .023\\ .037\\ .081\end{tabular} \\ \midrule
less letters                        & \begin{tabular}[c]{@{}l@{}}All\\ Rephrase\\ CoT\\ Gradual\end{tabular} & \begin{tabular}[c]{@{}l@{}}240\\ 42\\ 126\\ 69\end{tabular}     & \begin{tabular}[c]{@{}l@{}}207\\ 40\\ 119\\ 45\end{tabular}     & \begin{tabular}[c]{@{}l@{}}86.25\%\\ 95.24\%\\ 94.44\%\\ 65.22\%\end{tabular} & \begin{tabular}[c]{@{}l@{}}.338\\ .316\\ .319\\ .397\end{tabular}  & \begin{tabular}[c]{@{}l@{}}.078\\ .061\\ .068\\ .074\end{tabular} \\ \midrule
more letters                        & \begin{tabular}[c]{@{}l@{}}All\\ Rephrase\\ CoT\\ Gradual\end{tabular} & \begin{tabular}[c]{@{}l@{}}237\\ 45\\ 127\\ 62\end{tabular}     & \begin{tabular}[c]{@{}l@{}}210\\ 42\\ 123\\ 42\end{tabular}     & \begin{tabular}[c]{@{}l@{}}88.61\%\\ 93.33\%\\ 96.85\%\\ 67.74\%\end{tabular} & \begin{tabular}[c]{@{}l@{}}.374\\ .349\\ .359\\ .431\end{tabular}  & \begin{tabular}[c]{@{}l@{}}.081\\ .059\\ .075\\ .078\end{tabular} \\ \midrule
rhyming word                        & \begin{tabular}[c]{@{}l@{}}All\\ Rephrase\\ CoT\\ Gradual\end{tabular} & \begin{tabular}[c]{@{}l@{}}245\\ 47\\ 125\\ 70\end{tabular}     & \begin{tabular}[c]{@{}l@{}}219\\ 37\\ 115\\ 64\end{tabular}     & \begin{tabular}[c]{@{}l@{}}89.39\%\\ 78.72\%\\ 92.00\%\\ 91.43\%\end{tabular} & \begin{tabular}[c]{@{}l@{}}.234\\ .189\\ .198\\ .325\end{tabular}  & \begin{tabular}[c]{@{}l@{}}.079\\ .038\\ .049\\ .067\end{tabular} \\ \midrule
word before                         & \begin{tabular}[c]{@{}l@{}}All\\ Rephrase\\ CoT\\ Gradual\end{tabular} & \begin{tabular}[c]{@{}l@{}}233\\ 41\\ 125\\ 64\end{tabular}     & \begin{tabular}[c]{@{}l@{}}225\\ 39\\ 119\\ 64\end{tabular}     & \begin{tabular}[c]{@{}l@{}}96.57\%\\ 95.12\%\\ 95.20\%\\ 100.0\%\end{tabular} & \begin{tabular}[c]{@{}l@{}}.123\\ .088\\ .098\\ .195\end{tabular} & \begin{tabular}[c]{@{}l@{}}.049\\ .009\\ .012\\ .032\end{tabular} \\ \midrule
word not containing                 & \begin{tabular}[c]{@{}l@{}}All\\ Rephrase\\ CoT\\ Gradual\end{tabular} & \begin{tabular}[c]{@{}l@{}}234\\ 48\\ 125\\ 58\end{tabular}     & \begin{tabular}[c]{@{}l@{}}223\\ 47\\ 122\\ 51\end{tabular}     & \begin{tabular}[c]{@{}l@{}}95.30\%\\ 97.92\%\\ 97.60\%\\ 87.93\%\end{tabular} & \begin{tabular}[c]{@{}l@{}}.222\\ .177\\ .190\\ .337\end{tabular}  & \begin{tabular}[c]{@{}l@{}}.094\\ .059\\ .043\\ .115\end{tabular} \\ \midrule
all tasks                           & \begin{tabular}[c]{@{}l@{}}All\\ Rephrase\\ CoT\\ Gradual\end{tabular} & \begin{tabular}[c]{@{}l@{}}2429\\ 461\\ 1286\\ 652\end{tabular} & \begin{tabular}[c]{@{}l@{}}2186\\ 408\\ 1234\\ 514\end{tabular} & \begin{tabular}[c]{@{}l@{}}90.00\%\\ 88.50\%\\ 95.96\%\\ 78.83\%\end{tabular} & \begin{tabular}[c]{@{}l@{}}.296\\ .269\\ .279\\ .351\end{tabular}   & \begin{tabular}[c]{@{}l@{}}.070\\ .043\\ .048\\ .074\end{tabular} \\ 
\bottomrule
\end{tabular}%
}
\caption{
The distribution of correct paraphrases for each generation method across all tasks in \lmentry{}.
}
\label{table:paraphrases_correctness_lmentry}
% \end{adjustwidth}
\end{table*}

% Please add the following required packages to your document preamble:
% \usepackage{graphicx}
\begin{table*}[tb!]
\begin{adjustwidth}{0.5cm}{0.5cm}
\small
\resizebox{0.92\textwidth}{!}{%
\begin{tabular}{l|lccccc}
\toprule
\textbf{Benchmark \& Task}          & \textbf{Method}                                                        & \textbf{\begin{tabular}[c]{@{}c@{}}\#Auto \\ Paraphrases\end{tabular}}                                     & \textbf{\begin{tabular}[c]{@{}c@{}}\#Correct \\ Paraphrases\end{tabular}}                                  & \textbf{\begin{tabular}[c]{@{}l@{}}Correct \\ Ratio (\%)\end{tabular}}                                                   & \textbf{\begin{tabular}[c]{@{}l@{}}Model\\ Accuracy \\ (Avg.)\end{tabular}}                                & \textbf{\begin{tabular}[c]{@{}l@{}}Model\\ Accuracy \\ (Std.)\end{tabular}}                               \\
\hline
causal judgement                    & \begin{tabular}[c]{@{}l@{}}All\\ Rephrase\\ CoT\\ Gradual\end{tabular} & \begin{tabular}[c]{@{}l@{}}187\\ 50\\ 60\\ 76\end{tabular}      & \begin{tabular}[c]{@{}l@{}}153\\ 31\\ 55\\ 66\end{tabular}      & \begin{tabular}[c]{@{}l@{}}81.82\%\\ 62.00\%\\ 91.67\%\\ 86.84\%\end{tabular} & \begin{tabular}[c]{@{}l@{}}.477\\ .469\\ .452\\ .502\end{tabular}  & \begin{tabular}[c]{@{}l@{}}.034\\ .024\\ .023\\ .028\end{tabular} \\ \midrule
disambiguation qa                   & \begin{tabular}[c]{@{}l@{}}All\\ Rephrase\\ CoT\\ Gradual\end{tabular} & \begin{tabular}[c]{@{}l@{}}188\\ 50\\ 60\\ 77\end{tabular}      & \begin{tabular}[c]{@{}l@{}}177\\ 50\\ 50\\ 76\end{tabular}      & \begin{tabular}[c]{@{}l@{}}94.15\%\\ 100.0\%\\ 83.33\%\\ 98.70\%\end{tabular} & \begin{tabular}[c]{@{}l@{}}.412\\ .403\\ .357\\ .455\end{tabular}  & \begin{tabular}[c]{@{}l@{}}.049\\ .031\\ .022\\ .029\end{tabular} \\ \midrule
formal fallacies                    & \begin{tabular}[c]{@{}l@{}}All\\ Rephrase\\ CoT\\ Gradual\end{tabular} & \begin{tabular}[c]{@{}l@{}}184\\ 50\\ 56\\ 77\end{tabular}      & \begin{tabular}[c]{@{}l@{}}130\\ 19\\ 51\\ 59\end{tabular}      & \begin{tabular}[c]{@{}l@{}}70.65\%\\ 38.00\%\\ 91.07\%\\ 76.62\%\end{tabular} & \begin{tabular}[c]{@{}l@{}}.308\\ .326\\ .294\\ .313\end{tabular}  & \begin{tabular}[c]{@{}l@{}}.026\\ .027\\ .015\\ .027\end{tabular} \\ \midrule
geometric shapes                    & \begin{tabular}[c]{@{}l@{}}All\\ Rephrase\\ CoT\\ Gradual\end{tabular} & \begin{tabular}[c]{@{}l@{}}178\\ 50\\ 55\\ 72\end{tabular}      & \begin{tabular}[c]{@{}l@{}}171\\ 50\\ 53\\ 67\end{tabular}      & \begin{tabular}[c]{@{}l@{}}96.07\%\\ 100.0\%\\ 96.36\%\\ 93.06\%\end{tabular} & \begin{tabular}[c]{@{}l@{}}.163\\ .175\\ .153\\ .163\end{tabular}  & \begin{tabular}[c]{@{}l@{}}.020\\ .015\\ .019\\ .020\end{tabular} \\ \midrule
hyperbaton                          & \begin{tabular}[c]{@{}l@{}}All\\ Rephrase\\ CoT\\ Gradual\end{tabular} & \begin{tabular}[c]{@{}l@{}}155\\ 43\\ 36\\ 75\end{tabular}      & \begin{tabular}[c]{@{}l@{}}117\\ 32\\ 35\\ 49\end{tabular}      & \begin{tabular}[c]{@{}l@{}}75.48\%\\ 74.42\%\\ 97.22\%\\ 65.33\%\end{tabular} & \begin{tabular}[c]{@{}l@{}}.466\\ .467\\ .438\\ .484\end{tabular}  & \begin{tabular}[c]{@{}l@{}}.035\\ .020\\ .030\\ .034\end{tabular} \\ \midrule
logical deduction five objects      & \begin{tabular}[c]{@{}l@{}}All\\ Rephrase\\ CoT\\ Gradual\end{tabular} & \begin{tabular}[c]{@{}l@{}}189\\ 50\\ 59\\ 79\end{tabular}      & \begin{tabular}[c]{@{}l@{}}150\\ 47\\ 27\\ 75\end{tabular}      & \begin{tabular}[c]{@{}l@{}}79.37\%\\ 94.00\%\\ 45.76\%\\ 94.94\%\end{tabular} & \begin{tabular}[c]{@{}l@{}}.262\\ .239\\ .243\\ .283\end{tabular}  & \begin{tabular}[c]{@{}l@{}}.027\\ .009\\ .026\\ .015\end{tabular} \\ \midrule
logical deduction seven objects     & \begin{tabular}[c]{@{}l@{}}All\\ Rephrase\\ CoT\\ Gradual\end{tabular} & \begin{tabular}[c]{@{}l@{}}186\\ 50\\ 60\\ 75\end{tabular}      & \begin{tabular}[c]{@{}l@{}}145\\ 41\\ 31\\ 72\end{tabular}      & \begin{tabular}[c]{@{}l@{}}77.96\%\\ 82.00\%\\ 51.67\%\\ 96.00\%\end{tabular} & \begin{tabular}[c]{@{}l@{}}.236\\ .215\\ .219\\ .257\end{tabular}  & \begin{tabular}[c]{@{}l@{}}.026\\ .009\\ .028\\ .016\end{tabular} \\ \midrule
logical deduction three objects     & \begin{tabular}[c]{@{}l@{}}All\\ Rephrase\\ CoT\\ Gradual\end{tabular} & \begin{tabular}[c]{@{}l@{}}187\\ 50\\ 60\\ 76\end{tabular}      & \begin{tabular}[c]{@{}l@{}}147\\ 47\\ 27\\ 72\end{tabular}      & \begin{tabular}[c]{@{}l@{}}78.61\%\\ 94.00\%\\ 45.00\%\\ 94.74\%\end{tabular} & \begin{tabular}[c]{@{}l@{}}.359\\ .329\\ .317\\ .394\end{tabular}  & \begin{tabular}[c]{@{}l@{}}.044\\ .023\\ .030\\ .028\end{tabular} \\ \midrule
movie recommendation                & \begin{tabular}[c]{@{}l@{}}All\\ Rephrase\\ CoT\\ Gradual\end{tabular} & \begin{tabular}[c]{@{}l@{}}180\\ 47\\ 57\\ 75\end{tabular}      & \begin{tabular}[c]{@{}l@{}}164\\ 47\\ 50\\ 66\end{tabular}      & \begin{tabular}[c]{@{}l@{}}91.11\%\\ 100.0\%\\ 87.72\%\\ 88.00\%\end{tabular} & \begin{tabular}[c]{@{}l@{}}.348\\ .371\\ .323\\ .351\end{tabular}  & \begin{tabular}[c]{@{}l@{}}.036\\ .011\\ .040\\ .032\end{tabular} \\ \midrule
navigate                            & \begin{tabular}[c]{@{}l@{}}All\\ Rephrase\\ CoT\\ Gradual\end{tabular} & \begin{tabular}[c]{@{}l@{}}170\\ 50\\ 54\\ 65\end{tabular}      & \begin{tabular}[c]{@{}l@{}}152\\ 50\\ 54\\ 47\end{tabular}      & \begin{tabular}[c]{@{}l@{}}89.41\%\\ 100.0\%\\ 100.0\%\\ 72.31\%\end{tabular} & \begin{tabular}[c]{@{}l@{}}.386\\ .374\\ .388\\ .396\end{tabular}  & \begin{tabular}[c]{@{}l@{}}.019\\ .013\\ .021\\ .017\end{tabular} \\ \midrule
penguins in a table                 & \begin{tabular}[c]{@{}l@{}}All\\ Rephrase\\ CoT\\ Gradual\end{tabular} & \begin{tabular}[c]{@{}l@{}}183\\ 49\\ 59\\ 74\end{tabular}      & \begin{tabular}[c]{@{}l@{}}143\\ 37\\ 51\\ 54\end{tabular}      & \begin{tabular}[c]{@{}l@{}}78.14\%\\ 75.51\%\\ 86.44\%\\ 72.97\%\end{tabular} & \begin{tabular}[c]{@{}l@{}}.243\\ .250\\ .215\\ .265\end{tabular}  & \begin{tabular}[c]{@{}l@{}}.026\\ .014\\ .007\\ .018\end{tabular} \\ \midrule
ruin names                          & \begin{tabular}[c]{@{}l@{}}All\\ Rephrase\\ CoT\\ Gradual\end{tabular} & \begin{tabular}[c]{@{}l@{}}157\\ 50\\ 40\\ 66\end{tabular}      & \begin{tabular}[c]{@{}l@{}}143\\ 49\\ 35\\ 58\end{tabular}      & \begin{tabular}[c]{@{}l@{}}91.08\%\\ 98.00\%\\ 87.50\%\\ 87.88\%\end{tabular} & \begin{tabular}[c]{@{}l@{}}.254\\ .252\\ .250\\ .258\end{tabular}  & \begin{tabular}[c]{@{}l@{}}.016\\ .015\\ .019\\ .013\end{tabular} \\ \midrule
salient translation error detection & \begin{tabular}[c]{@{}l@{}}All\\ Rephrase\\ CoT\\ Gradual\end{tabular} & \begin{tabular}[c]{@{}l@{}}136\\ 47\\ 25\\ 63\end{tabular}      & \begin{tabular}[c]{@{}l@{}}128\\ 46\\ 25\\ 56\end{tabular}      & \begin{tabular}[c]{@{}l@{}}94.12\%\\ 97.87\%\\ 100.0\%\\ 88.89\%\end{tabular} & \begin{tabular}[c]{@{}l@{}}.191\\ .185\\ .192\\ .196\end{tabular}  & \begin{tabular}[c]{@{}l@{}}.015\\ .011\\ .007\\ .019\end{tabular} \\ \midrule
snarks                              & \begin{tabular}[c]{@{}l@{}}All\\ Rephrase\\ CoT\\ Gradual\end{tabular} & \begin{tabular}[c]{@{}l@{}}162\\ 50\\ 37\\ 74\end{tabular}      & \begin{tabular}[c]{@{}l@{}}152\\ 50\\ 37\\ 64\end{tabular}      & \begin{tabular}[c]{@{}l@{}}93.83\%\\ 100.0\%\\ 100.0\%\\ 86.49\%\end{tabular} & \begin{tabular}[c]{@{}l@{}}.405\\ .396\\ .410\\ .408\end{tabular}  & \begin{tabular}[c]{@{}l@{}}.025\\ .024\\ .030\\ .021\end{tabular} \\ \midrule
sports understanding                & \begin{tabular}[c]{@{}l@{}}All\\ Rephrase\\ CoT\\ Gradual\end{tabular} & \begin{tabular}[c]{@{}l@{}}173\\ 48\\ 57\\ 67\end{tabular}      & \begin{tabular}[c]{@{}l@{}}137\\ 31\\ 49\\ 56\end{tabular}      & \begin{tabular}[c]{@{}l@{}}79.19\%\\ 64.58\%\\ 85.96\%\\ 83.58\%\end{tabular} & \begin{tabular}[c]{@{}l@{}}.461\\ .469\\ .453\\ .463\end{tabular}  & \begin{tabular}[c]{@{}l@{}}.052\\ .051\\ .068\\ .035\end{tabular} \\ \midrule
all tasks                           & \begin{tabular}[c]{@{}l@{}}All\\ Rephrase\\ CoT\\ Gradual\end{tabular} & \begin{tabular}[c]{@{}l@{}}2615\\ 734\\ 775\\ 1091\end{tabular} & \begin{tabular}[c]{@{}l@{}}2209\\ 627\\ 630\\ 937\end{tabular}  & \begin{tabular}[c]{@{}l@{}}84.47\%\\ 85.42\%\\ 81.29\%\\ 85.88\%\end{tabular} & \begin{tabular}[c]{@{}l@{}}.331\\ .327\\ .314\\ .346\end{tabular}  & \begin{tabular}[c]{@{}l@{}}.035\\ .025\\ .030\\ .029\end{tabular} \\
\bottomrule
\end{tabular}%

}
\caption{The distribution of correct paraphrases for each generation method across all tasks in \bbh{}.}
\label{table:paraphrases_correctness_bbh}
\end{adjustwidth}
\end{table*}

\subsection{Comparing Different Instruction Templates with Kendall's $\tau$ Rank Disagreements}
\label{sec:tau-comparison}
Tables~\ref{tab:tau_lmentry}
, \ref{tab:tau_bbl}, and~\ref{tab:tau_bbh} present the Kendall $\tau$ values of representative examples from all benchmarks with Kendall $\tau$ values that are significantly different from 0. i.e., notable variations in rankings of models for two paraphrases of the same task instruction.

\begin{table*}[bt!]
\small
\centering
%\resizebox{textwidth}{!}{
\begin{tabular}{lp{5cm}p{5cm}c}
\toprule
Task & Instruction Template \#1 & Instruction Template \#2 & $\tau$ \\ \midrule
 all words from category & 
 Can you confirm if the list [\{$words$\}] consists solely of \{$category$\}? Please respond with either "yes" or "no".
& 
Determine whether all the words in a given list belong to a specific category. The category is represented by the keyword \{$category$\}, and the list of words is represented by the keyword \{$words$\}. Answer the question with either 'yes' or 'no'.
Category: \{$category$\}
Words: \{$words$\}
Output:
& 0.029 \\
  any words from category & Is \{$category$\} represented by any of these words \{$words$\}? Respond with either 'yes' or 'no'.
  & Given a list of words, determine if any of them belong to a specific category. Respond with either "yes" or "no".
Words: \{$words$\}
Category: \{$category$\}
Output: & -0.200 \\
 ends with word & 
Provide a sentence that finishes with the term \{$word$\}. & 
Generate a sentence that ends with a specific word. Try to create a coherent sentence that effectively uses the provided word.
Word: \{$word$\}
Sentence: & -0.018 \\
 first alphabetically& 
 Which word comes first alphabetically, ``\{$word1$\}'' or ``\{$word2$\}''?
 & Please determine which of the two provided words is the first one alphabetically. The two words to be compared are denoted by placeholders \{$word1$\} and \{$word2$\}.
Word 1: \{$word1$\}
Word 2: \{$word2$\}
Output: The first word alphabetically is
& -0.095 \\
 homophones & 
 Can you tell me which word, \{$word1$\} or \{$word2$\}, sounds like \{$query$\}? & 
 Given two words, determine which one is a homophone or sounds more like a query word.
Query word: \{$query$\}
Word 1: \{$word1$\}
Word 2: \{$word2$\}
The word that sounds more like {query} is:
& 0.087 \\
 less letters & 
 Which of \{$word1$\} and \{$word2$\} has fewer letters? 
 & Compare two words and determine which one has fewer letters. The words are represented by the keywords \{$word1$\} and \{$word2$\}. Provide the keyword of the word with fewer letters.
word1: \{$word1$\}
word2: \{$word2$\}
Output keyword:
& -0.128 \\
 more letters & 
 Please compare the length of ``\{$word1$\}'' and ``\{$word2$\}'' and provide the longer word.
 & Write a program that compares the length of two words and determines which one has more letters. Your program should take two words as input and output the word with more letters. 
Word 1: \{$word1$\}
Word 2: \{$word2$\}
Output:
& -0.085 \\
 rhyming word & 
 What is a word that rhymes with `\{$query$\}', `\{$word1$\}' or `\{$word2$\}'? & 
Given a query word and two candidate words, determine which candidate word rhymes with the query word. Your response should be the candidate word that rhymes with the query word. 
Query word: \{$query$\}
Candidate word 1: \{$word1$\}
Candidate word 2: \{$word2$\}
Output word:& 0.090 \\
 word before & 
 Locate the word that comes immediately before `\{$word$\}' in the given sentence `\{$sentence$\}'
& Given a sentence and a target word, identify the word that immediately precedes the target word in the sentence.
Sentence: \{$sentence$\}
Target word: \{$word$\}
The word that comes right before \{$word$\} in the sentence is:
& -0.099 \\
 word not containing & 
 Create a term that does not have the inclusion of the letter ``\{$letter$\}''.
 & Write a word that does not contain the letter ``\{$letter$\}''.
Letter: \{$letter$\}
Output word: & -0.010 \\

\bottomrule

\end{tabular}%
%}
\caption{Kendall $\tau$ values of the disagreement between ranks on models from example paraphrases for each task in \lmentry{}.}
\label{tab:tau_lmentry}
\end{table*}

\begin{table*}[bt!]
\begin{adjustwidth}{-1cm}{-1cm}
\small
\centering
%\resizebox{textwidth}{!}{

\begin{tabular}{@{}p{1.5cm}p{7.5cm}p{7.5cm}c@{}}
\toprule
Task & Instruction Template \#1 & Instruction Template \#2 & $\tau$ \\ \midrule
  causal judgement    & You are required to give your opinion on the following question about causation: \{$question$\}. You must select either ``yes'' or ``no''. & Given a scenario, determine whether a typical person would attribute causality to a certain factor or not. Answer with ``yes'' or ``no''.
Scenario: \{$question$\}
Answer: & 0.183 \\
 disambiguation qa   & Q: For the given sentence, identify the antecedent of the ambiguous pronoun or state that it is ambiguous.
Sentence: \{$sentence$\}
Choose the option that correctly identifies the antecedent of the pronoun:
\{$options$\}
A: & Please clarify the meaning of the following sentence by selecting the option that correctly identifies the antecedent of the pronoun or state if it is ambiguous.
Sentence: \{$sentence$\}
Options:
\{$options$\}
Output: & 0.164 \\
 formal fallacies   & Q: ``Classify the argument as either a formal fallacy or deducively valid. The explicitly stated premises are \{$input$\}.''
Options:
- deductively valid
- formal fallacy & Given a set of explicitly stated premises, determine whether the argument is deductively valid or a formal fallacy. Respond with ``valid'' or ``invalid''.
Premises and conclusion: \{$input$\}
Output: & -0.264 \\
  geometric shapes  & Q: Identify the name of the geometric shape represented by the following SVG path element: \{$svg\_path\_element$\}.
Options:
\{$options$\}
A: & From the given options \{$options$\}, select the name of the geometric shape that is represented by \{$svg\_path\_element$\}. & -0.267 \\
 hyperbaton   & Order the adjectives correctly before a noun in English sentences, following the pattern of ``[1. opinion] [2. size] [3. age] [4. shape] [5. color] [6. origin] [7. material] [8. purpose] noun''. You will be presented with a multi-choice format question asking which sentence has the correct adjective order, with options provided.
Which of the following sentences has the correct adjective order?
\{$options$\} & Identify the sentence that has the correct order of adjectives in English. Choose the sentence that has the correct order of adjectives. 
Options:
\{$options$\}
Output: & 0.019 \\
 logical deduction five objects    & In this logical deduction task named logical deduction five objects, you will be given a set of paragraphs describing a set of five objects arranged in a fixed order. The statements are logically consistent within each paragraph. Your task is to choose the correct option from the given options. The options are \{$options$\}. The paragraph is \{$paragraph$\}. & Deduce the order of a sequence of five objects based on given logical statements. You will be given a set of logical statements and multiple choices for the order of the objects. Choose the correct order based on the given statements.
Statements: \{$paragraph$\}
Options:
\{$options$\}
Output: & 0.264 \\
 logical deduction seven objects    & Your task is to solve a logical deduction task which requires you to deduce the order of a sequence of objects. The task consists of a set of paragraphs, each describing a set of seven objects arranged in a fixed order. The statements are logically consistent within each paragraph. You will also be provided with multiple options to choose from. The options are represented by \{$options$\}. You should choose the correct option based on the information provided in the paragraph, which is represented by \{$paragraph$\}. & Deduce the order of a sequence of seven objects based on given statements. Use the provided options to answer each question.
Statements: \{$paragraph$\}
Options:
\{$options$\}
Output: & 0.133 \\
  logical deduction three objects   & Deduce the order of a sequence of three objects based on the logically consistent statements provided in the following \{$paragraph$\}. Choose the correct order from the given \{$options$\}. & Deduce the order of a sequence of three objects based on given statements and choose the correct option among multiple choices.
Statements: \{$paragraph$\}
Options:
\{$options$\}
Output: & 0.056 \\
 movie recommendation    & Q: Can you suggest a movie similar to \{$movie\_list$\}?
Please choose from the following options:
\{$options$\}
A: & Based on a list of movies, recommend a similar movie from a set of options. Choose the option that best matches the given list.
List of movies: \{$movie\_list$\}
Options:
\{$options$\}
Output: & -0.018 \\
  navigate  & Q: Would someone following \{$instructions$\} end up back at the starting point?
Options:
- Yes
- No
A: & Classify whether a series of navigation instructions will lead to the starting point or not. Provide either ``yes'' or ``no'' as the output. 
Instructions: \{$instructions$\}
Output: & 0.294 \\
  penguins in a table   & Please answer the following question about the table of penguins: \{$question$\} The table has a header and each subsequent line represents a penguin with attributes: name, age, height (cm), weight (kg). \{$table\_description$\} You can choose from the following options: \{$options$\} & Given a table of penguins and their attributes, answer multiple choice questions about the penguins. The prompt will include a description of the table and several options to choose from.
Table: \{$table\_description$\}
Question prompt: \{$question$\}
Options: 
\{$options$\}
Output: & 0.241 \\
  ruin names  & Which of the following options is a funny way to ``ruin'' the name of \{$artist\_or\_movie\_name$\}?
Choose from the following:
\{$options$\} & Choose the option that best 'ruins' the \{$artist\_or\_movie\_name$\}:
Options:
\{$options$\}
Answer: & 0.075 \\
  salient translation error detection & Q: Identify the type of error in the given English translation of a German source sentence. The error will belong to one of the following categories: Named Entities, Numerical Values, Modifiers or Adjectives, Negation or Antonyms, Facts, or Dropped Content. The source sentence is \{$source$\}, and its translation is \{$translation$\}. From the options below, select the category that best describes the error.
Options:
\{$options$\} & Given an English translation of a German source sentence, identify the type of error present in the translation. The error can be one of the following types: Named Entities, Numerical Values, Modifiers or Adjectives, Negation or Antonyms, Facts, or Dropped Content. You must select the correct answer from the given options in a multi-choice format.
German source sentence: \{$source$\}
English translation: \{$translation$\}
Options:
\{$options$\} & 0.389 \\
  snarks & Determine which of two sentences is sarcastic. The format is multi-choice and the prompt asks ``which statement is sarcastic?'' with two options provided. The correct option contains a taste of irony and satire. 
Options:
\{$options$\}
Output: & Given a question asking which statement is sarcastic and a list of options to choose from, determine which of the options is the sarcastic one.
Question: ``which statement is sarcastic?''
Options: 
\{$options$\}
Output: & 0.22 \\
  sports understanding  & Please classify the sentence ``\{$sentence$\}'' as either plausible or not plausible in the context of sports. & Is the following sentence plausible? \{$sentence$\}
Answer with either ``yes'' or ``no''.
Output: & -0.245 \\ 
\bottomrule

\end{tabular}%

%}
\caption{Kendall $\tau$ values of the disagreement between ranks on models from example paraphrases for each task in \bbh{}.}
\label{tab:tau_bbh}
\end{adjustwidth}
\end{table*}

\begin{table*}[bt!]
\begin{adjustwidth}{-1cm}{-1cm}
\small
\centering
%\resizebox{textwidth}{!}{
\begin{tabular}{p{1.5cm}p{7cm}p{7cm}c}
\toprule
Task & Instruction Template \#1 & Instruction Template \#2 & $\tau$ \\ \midrule
 bbq lite    & You are examined with your ability on social fairness by answering questions that contain bias content including: age, disability, gender, nationality, physical appearance, race ethnicity, religion, social status, and sexual orientation. \{$question$\}
Choose the most appropriate answer from: 
A) \{$choiceA$\}
B) \{$choiceB$\}
C) \{$choiceC$\}. & We are running a test for social biases. We will give you a question and a series of multiple-answers (A, B, C). Please choose from among the answers.

Question: \{$question$\}
A: \{$choiceA$\}
B: \{$choiceB$\}
C: \{$choiceC$\}

Answer: & 0.222 \\
    code line description    & If you are an experienced code reviewer, please give an English language description of Python code\{$question$\}. Which is the most suitable? A.  \{$choiceA$\} B.  \{$choiceB$\} C.  \{$choiceC$\} D.  \{$choiceD$\}

Answer: & You are given a simple line of Python code \{$question$\}. Try to find out its English equivalency from the following short sentences: A) \{$choiceA$\}, B) \{$choiceB$\} C) \{$choiceC$\}, D) \{$choiceD$\}. The equivalent sentence is: & 0.333 \\
   conceptual combinations     & You are a linguistic expert that knows most of the concepts and combinations of words. Now, answer the following question: \{$context$\} Question: \{$question$\} (A) \{$choiceA$\} (B) \{$choiceB$\} (C) \{$choiceC$\} (D) \{$choiceD$\}
Your answer is: & Question: \{$question$\}
The options are: 
A. \{$choiceA$\}
B. \{$choiceB$\}
C. \{$choiceC$\}
D. \{$choiceD$\}
Here is a context to help you answer the question: \{$context$\}. Choose the best answer from ``A'', ``B'', ``C'', ``D''. & 0.182 \\
    hindu knowledge   & In this task, you have to select the option that best answers the question given your knowledge about Hindu mythology.
Question: \{$question$\}
A.  \{$choiceA$\} B.  \{$choiceB$\} C.  \{$choiceC$\} D.  \{$choiceD$\}
Answer: among A, B, C, and D, the best choice is & \{$question$\}

A: \{$choiceA$\} B: \{$choiceB$\} C: \{$choiceC$\} D: \{$choiceD$\}
With your expertise inhindu mythology, provide the correct answer: & 0.444 \\
   known unknown   & Verify if the question is unknown, choose your answer from options:
Question: \{$question$\}
Options:
A: \{$choiceA$\}
B: \{$choiceB$\}
Answer: & Question: \{$question$\}
To avoid hallucination, if the answer to this question is unknown, output ``B'', otherwise output ``A'' & -0.029 \\
    language identification   & Please read the following sentence, then choose from the options which language you think it most likely came from. Your answer should be ``A'', ``B'', ``C'', ``D'', ``E'', ``F'', ``G'', ``H'', ``I'', ``J'', or ``K''
Sentence: \{$question$\}
Options:
A: \{$choiceA$\}
B: \{$choiceB$\}
C: \{$choiceC$\}
D: \{$choiceD$\}
E: \{$choiceE$\}
F: \{$choiceF$\}
G: \{$choiceG$\}
H: \{$choiceH$\}
I: \{$choiceI$\}
J: \{$choiceJ$\}
K: \{$choiceK$\}
Answer: & Please give the language used in the following sentence. Each sentence will give five options, please output the corresponding option (i.e. A, B, C, D, E, F, G, H, I, J, or K) to represent the corresponding answer.

Sentence: \{$question$\}
Options: & 0.028 \\
     logic grid puzzle   & You are given a logic grid puzzle to test your sense of space and positions. You are given a context and some clues to pick the correct answer from the options to answer a question.Context: \{$context$\}
\{$clues$\}
Question: \{$question$\}
Options:
(A) \{$choiceA$\}
(B) \{$choiceB$\}
(C) \{$choiceC$\}
(D) \{$choiceD$\}
(E) \{$choiceE$\}
Answer: & You are a master at solving logic grid puzzles. Solve this: \{$context$\}

\{$clues$\}

\{$question$\} & 0.327 \\
    logical deduction   & Given the following text describing the correct order of five objects, select the option from (A, B, C, D or E) that is consistent with the text.

text: \{$question$\}\{$options$\}

answer: & The following text describes the arrangement order of five objects. Please read the text and choose the one from the options that matches the logic of the text description. Your answer should be ``A'', ``B'', ``C'', ``D'' or ``E''.
Text: \{$question$\}\{$options$\} Answer: & 0.667 \\
    novel concepts   & You are given three objects \{$question$\}, choose the option from below where the objects share the greatest similarity. A. \{$choiceA$\} B. \{$choiceB$\} C. \{$choiceC$\} D. \{$choiceD$\} E. \{$choiceE$\} & \{$question$\}
Pick the most correct description from:
A.\{$choiceA$\}
B. \{$choiceB$\}
C. \{$choiceC$\}
D. \{$choiceD$\}
E. \{$choiceE$\}
My answer is: & 0.400 \\
    play dialog    & Now you are a dramatist. The following transcripts of dialogues are taken from Shakespeare plays, but the transcripts do not mark who said what.  Your task is to identify whether the sentences in question were spoken by the same or different people. Here is the play:
\{$play$\}
Question: In the preceding dialogue, were the lines \{$line1$\} and \{$line2$\} spoken by the same person or different people? Please just give a short answer: same or different.

Your Answer: & In the context of the Shakespeare play, \{$play$\}, assess the given dialogue transcripts. Determine whether the sentences \{$line1$\} and \{$line2$\} were spoken by a single person or by different people.
Answer: & -0.638 \\
    strange stories    & Given a story, answer whether the question is true or false.
\{$context$\}
Q: \{$question$\}
A: & Image you are taking a psychology test. Please read the given story and answer the question. Please answer ``yes'' or ``no''.
Story: \{$context$\}
Q: \{$question$\}
A: & 0.310 \\
    strategic qa    & Reason about the answer to the question. \{$question$\} & Please answer the following question, you should think step by step, but please use ``yes'' or ``no'' to answer.Question: \{$question$\}Answer: & -0.085 \\
    vitaminc fact verification    & Input: \{$claim$\}
Verify the factually of the claim based on the following context
\{$context$\}

- ``True'' if the claim is factually correct
- ``False'' if the claim is factually incorrect
- ``Neither'' if the factuality cannot be determined. Output you answer with one of ``True'', ``False'', or ``Neither''. Answer: & Context: \{$context$\}
Now classify this claim into one of 'True', 'False', or 'Neither'.
\{$claim$\} & 0.556 \\
     winowhy   & Read the following reasoning about who a particular pronoun refers to: \{$question$\}
Is the reasoning correct? & Read the following reasoning, and answer if its correct or incorrect. \{$question$\} & -0.056 \\ 
\bottomrule

\end{tabular}%
%}
\caption{Kendall $\tau$ values of the disagreement between ranks on models from example paraphrases for each task in \bbl{}.}
\label{tab:tau_bbl}
\end{adjustwidth}
\end{table*}
}

\subsection{Model Performance Differences with Minimal Paraphrasing Edit Distance}
\label{sec:appendix_min_edit_dist}
\remove{
Figure~\ref{fig:edit_dist_pairs} depicts the average performance differences between various LLMs when small edits are made to the instruction templates.
\begin{figure*}[!htbp]
\includegraphics[width=\textwidth]{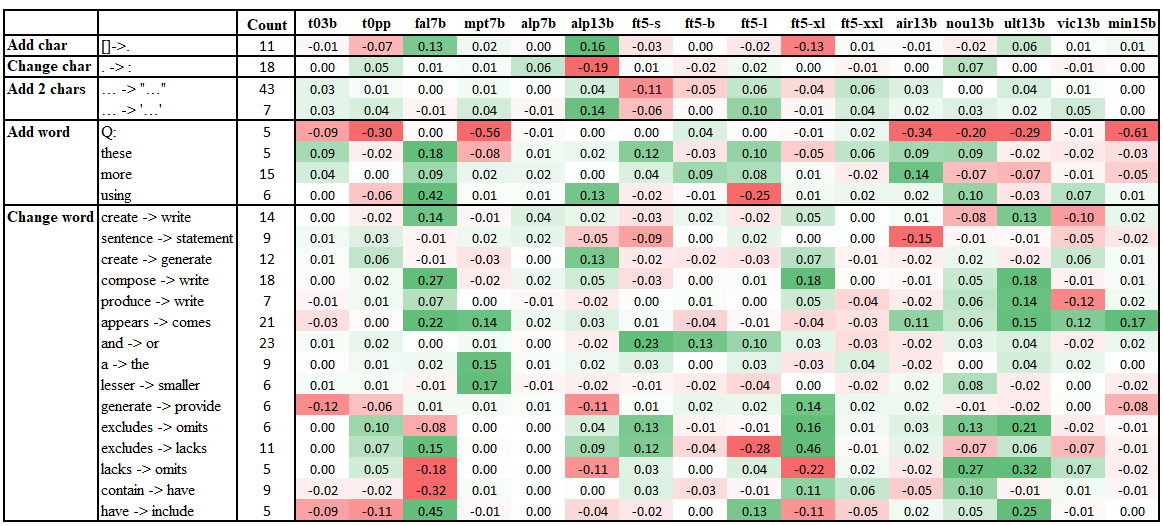}
\caption{\label{fig:edit_dist_pairs}
Average performance differences between various models when small edits are made to the prompts (e.g., substituting 'excludes' with 'lacks'). The count column describes the number of tasks for which this edit was relevant. 
}\end{figure*}
}
% In addition, 
Table~\ref{tab:min_edit_dist_max_diff} shows representative examples of instruction template pairs with very minor differences but notable variations in performance.
% Please add the following required packages to your document preamble:
% \usepackage{graphicx}
% \usepackage[table,xcdraw]{xcolor}
% Beamer presentation requires \usepackage{colortbl} instead of \usepackage[table,xcdraw]{xcolor}
\begin{table*}[!t]{
\begin{adjustwidth}{-1cm}{-1cm}
% \resizebox{\textwidth}{!}{%
\centering
\small
\begin{tabular}{|p{1.1cm}|c|p{5cm}|c|p{5cm}|c|c|}
\toprule
\textbf{Change}               & \textbf{Model}     & \textbf{P1}                                                                                                       & \textbf{Acc.} & \textbf{P2}                                                                                                          & \textbf{Acc.} & \textbf{Diff.}               \\ \hline
`.' --\textgreater `:'        & nous-hermes    & Create a word that does not include the letter   ``\{letter\}''.                                                    & .04          & Create a word that does not include the letter   ``\{letter\}''\textbf{\textit{:}}                                                       & .65          & {\color[HTML]{00B050} +.62} \\
                              & alpaca-13b         & Create a sentence that concludes with the term   ``\{word\}''.                                                      & .61          & Create a sentence that concludes with the term   ``\{word\}''\textbf{\textit{:}}                                                         & .19          & {\color[HTML]{C00000} -.42} \\ \hline
+ `.'                       & alpaca-13b         & Write a word that lacks the letter ``\{letter\}''                                                                   & .04          & Write a word that lacks the letter ``\{letter\}''\textbf{\textit{.}}                                                                     & .42          & {\color[HTML]{00B050} +.38} \\
                              % & falcon-7b & Write a word that lacks the letter ``\{letter\}''                                                                   & .19          & Write a word that lacks the letter ``\{letter\}''\textbf{\textit{.}}                                                                     & .50          & {\color[HTML]{00B050} +.31} \\
                              & flan-t5-xl         & Write a word that omits the letter ``\{letter\}''                                                                   & .77          & Write a word that omits the letter ``\{letter\}''\textbf{\textit{.}}                                                                     & .54          & {\color[HTML]{C00000} -.23} \\ \hline
+ `using'                   & flan-t5-large      & Your task is to write a word without the letter   ``\{letter\}''.                                                   & .46          & Your task is to write a word without \textbf{\textit{using}} the letter   ``\{letter\}''.                                                & .12          & {\color[HTML]{C00000} -.35} \\
                              & falcon-7b & Write a word without the letter \{letter\}.\textbackslash{}nOutput word:                                          & .12          & Write a word without \textbf{\textit{using}} the letter \{letter\}.\textbackslash{}nOutput word:                                       & .35          & {\color[HTML]{00B050} +.23} \\
                              % & flan-t5-large      & Write a word without the letter \{letter\}.\textbackslash{}nOutput word:                                          & .73          & Write a word without \textbf{\textit{using}} the letter \{letter\}.\textbackslash{}nOutput word:                                       & .50          & {\color[HTML]{C00000} -.23} \\ 
                              \hline
omits --\textgreater lacks    & ultralm-13b        & Write a word that \textbf{\textit{omits}} the letter ``\{letter\}''.                                                                  & .62          & Write a word that \textbf{\textit{lacks}} the letter ``\{letter\}''.                                                                     & .19          & {\color[HTML]{C00000} -.42} \\
                              % & falcon-7b & Write a word that \textbf{\textit{omits}} the letter ``\{letter\}''.                                                                  & .19          & Write a word that \textbf{\textit{lacks}} the letter ``\{letter\}''.                                                                     & .50          & {\color[HTML]{00B050} +.31} \\
                              & flan-t5-xl         & Write a word that \textbf{\textit{omits}} the letter ``\{letter\}''.                                                                  & .54          & Write a word that \textbf{\textit{lacks}} the letter ``\{letter\}''.                                                                     & .81          & {\color[HTML]{00B050} +.27} \\ \hline
\begin{tabular}[c]{@{}l@{}}contain \\ --\textgreater have\end{tabular}   & falcon-7b & Write a word that does not \textbf{\textit{contain}} the letter   ``\{letter\}''.                                                     & .81          & Write a word that does not \textbf{\textit{have}} the letter   ``\{letter\}''.                                                           & .19          & {\color[HTML]{C00000} -.62} \\
                              % & falcon-7b & Write a word that does not \textbf{\textit{contain}} the letter   ``\{letter\}''.                                                     & .81          & Write a word that does not \textbf{\textit{have}} the letter   ``\{letter\}''.                                                           & .27          & {\color[HTML]{C00000} -.54} \\
                              & flan-t5-xxl        & Please write a word that does not \textbf{\textit{contain}} the letter   ``\{letter\}''.                                              & .62          & Please write a word that does not \textbf{\textit{have}} the letter   ``\{letter\}''.                                                    & .88          & {\color[HTML]{00B050} +.27} \\ \hline
\begin{tabular}[c]{@{}l@{}}include \\ --\textgreater have\end{tabular}  & falcon-7b & Write a word that does not \textbf{\textit{include}} the letter   ``\{letter\}''.                                                     & .81          & Write a word that does not \textbf{\textit{have}} the letter   ``\{letter\}''.                                                           & .19          & {\color[HTML]{C00000} -.62} \\
                              & flan-t5-xl         & Write a word that does not \textbf{\textit{include}} the letter   ``\{letter\}''.                                                     & .42          & Write a word that does not \textbf{\textit{have}} the letter   ``\{letter\}''.                                                           & .73          & {\color[HTML]{00B050} +.31} \\
                              % & falcon-7b & Please write a word that does not \textbf{\textit{include}} the letter   ``\{letter\}''.                                              & .77          & Please write a word that does not \textbf{\textit{have}} the letter   ``\{letter\}''.                                                    & .35          & {\color[HTML]{C00000} -.42} \\
                              & ultralm-13b        & Please write a word that does not \textbf{\textit{include}} the letter   ``\{letter\}''.                                              & .46          & Please write a word that does not \textbf{\textit{have}} the letter   ``\{letter\}''.                                                    & .12          & {\color[HTML]{C00000} -.35} \\ \hline
excludes --\textgreater lacks & flan-t5-large      & Write a word that \textbf{\textit{excludes}} the letter ``\{letter\}''.                                                               & .54          & Write a word that \textbf{\textit{lacks}} the letter ``\{letter\}''.                                                                     & .12          & {\color[HTML]{C00000} -.42} \\
                              & flan-t5-xl         & Write a word that \textbf{\textit{excludes}} the letter ``\{letter\}''.                                                               & .19          & Write a word that \textbf{\textit{lacks}} the letter ``\{letter\}''.                                                                     & .81          & {\color[HTML]{00B050} +.62} \\
                              % & flan-t5-xl         & Write a word that \textbf{\textit{excludes}} the letter ``\{letter\}''                                                                & .46          & Write a word that \textbf{\textit{lacks}} the letter ``\{letter\}''                                                                      & .88          & {\color[HTML]{00B050} +.42} \\ 
                              \bottomrule
\end{tabular}% \\
\caption{Representative examples of instruction template pairs from \lmentry{} with very minor differences but notable variations in performance (open-source models).}
\label{tab:min_edit_dist_max_diff}
\end{adjustwidth}
}\end{table*}

\remove{
\subsection{BBL Analysis}
\label{sec:bbl_analysis}
This subsection consists of an additional analysis of the BBL benchmark that was not detailed in the main body of the paper.
Table~\ref{tab:tasks_info2} presents the Kendall's W values and the Friedman test p-values that demonstrate a low correlation between the ranks of the models for different instruction templates and reveal similar inconsistencies as observed with automated paraphrases in other benchmarks.}

\subsection{Model and Task Performance Divergence}
Figures~\ref{fig:divergence_bbh} \&~\ref{fig:divergence_bbl} show the deviation of the original instruction template from the average performance calculated over the generated instruction templates of several models for all of the BBH and BBL tasks respectively.

\begin{figure}[p]
\includegraphics[width=\linewidth]{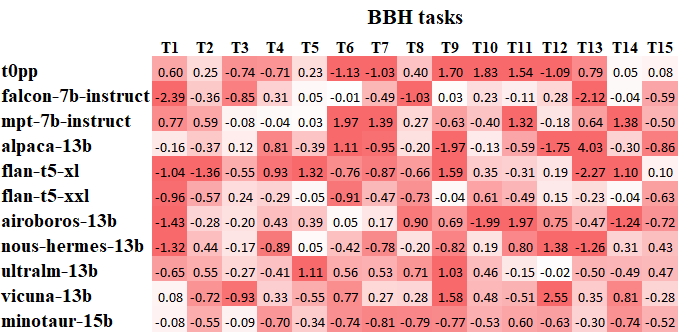}
\caption{\label{fig:divergence_bbh}
{Model and task performance divergence. For each task, this table shows the number of standard deviations by which the performance of each model on the original prompts deviates from the average model performance. Dark red cells indicate substantial divergence values exceeding one standard deviation.}
}\end{figure}

\begin{figure}[p]
\includegraphics[width=\linewidth]{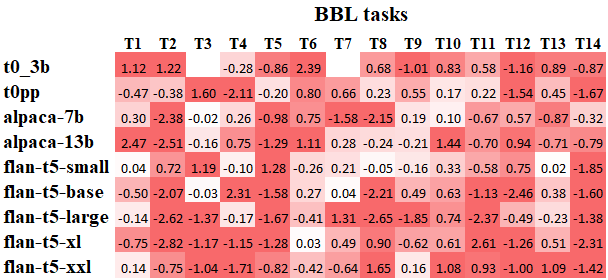}
\caption{\label{fig:divergence_bbl}
{Model and task performance divergence. For each task, this table shows the number of standard deviations by which the performance of each model on the original prompts deviates from the average model performance. Dark red cells indicate substantial divergence values exceeding one standard deviation.}
}\end{figure}

\remove{
% Noise in automatic paraphrases have no impact on metric-based model rankings:
\begin{table}[!htbp]
% \centering
% \small
\resizebox{1.02\columnwidth}{!}{%
\begin{tabular}{lcccc}
% \hline \textbf{Benchmark} & 
\toprule
\textbf{Benchmark \& Task} & \textbf{MaxP} & \textbf{AvgP}& \textbf{Sat} & \textbf{Combined}
\\ \hline
\textbf{\lmentry{}}  \\
 $\quad$ all words from category & .958 & .967 & .950 & .900\\
 $\quad$ any words from category & .979 & .967 & .983 & .983\\
 $\quad$ ends with word &  .104 & .967 & .050 & .517\\
 $\quad$ first alphabetically  & 1.00 & .950 & .933 & .950\\
 $\quad$ homophones  & .945 & 1.00 & .900 & .933\\
 $\quad$ less letters  & .983 & 1.00 & .917 & .967\\
 $\quad$ more letters  & .970 & .983 & .917 & .983\\
 $\quad$ rhyming word  & 1.00 & .967 & .983 & .967\\
 $\quad$ word before  & 1.00 & 1.00 & .983 & 1.00\\
 $\quad$ word not containing  & .836 & .967 & .783 & .850\\
  
\midrule

\textbf{\bigbenchhard{}} \\ 
$\quad$ causal judgement  & 1.00 & 1.00 & 1.00 & 1.00\\
$\quad$ disambiguation qa  &  1.00 & 1.00 & .964 & 1.00\\
$\quad$ formal fallacies  &   .991 & .927 & .818 & .855\\
$\quad$ geometric shapes  & 1.00 & .964 & 1.00 & .964\\
$\quad$ hyperbaton  &  .953 & 1.00 & .927 & .964\\
$\quad$ logical deduction five objects  & 1.00 & .964 & .855 & .964\\
$\quad$ logical deduction seven objects  & 1.00 & 1.00 & .964 & .964\\
$\quad$ logical deduction three objects  &  1.00 & .964 & .891 & .964\\
$\quad$ movie recommendation  & .954 & .927 & .891 & .964\\
$\quad$ navigate  &   .964 & 1.00 & 1.00 & .964\\
$\quad$ penguins in a table  & 1.00 & 1.00 & .891 & 1.00\\
$\quad$ ruin names  & 1.00 & 1.00 & .964 & .891\\
$\quad$ salient translation error detection  & 1.00 & 1.00 & 1.00 & 1.00\\
$\quad$ snarks  & 1.00 & 1.00 & .964 & 1.00\\
$\quad$ sports understanding  & 1.00 & 1.00 & .964 & 1.00\\

\bottomrule
\end{tabular}
}
\caption{\label{tab:metric_rankings_comparisson} Kendall's Tau model ranking comparisons before and after removal of incorrect paraphrases. Results show near-perfect to perfect agreement across all tasks, except for \lmentry{}'s “ends with word” task.
}
% \mnote{DAN: we can cite this work https://aclanthology.org/2022.naacl-main.167.pdf as they say  "We find that models can learn just as fast with many prompts that are intentionally irrelevant or even pathologically misleading as they do with constructively “good” prompts.". this might also be inline with \citet{sun2023evaluating} (wrong templates similar to templates observed in training preformed as better instruction templates than correct and unobserved templates)}
\end{table}

\subsection{Average Model Ranks for Each Metric Across All Tasks}

Tables~\ref{tab:model_rankings_avg_new_lmentry}, \ref{tab:model_rankings_avg_new_bbh} present the average model ranks for each metric across all tasks in \lmentry{} and \bbh{} respectively. 
\flanxxl{} emerges as the top performer for all metrics in both benchmarks. Minotaur is at the bottom of the performance spectrum across all evaluated models in \bbh{}.

\subsection{Analysis of Origin Generation Method of Optimal Paraphrases}
Our analyses for the origin of the optimal paraphrases used by each model, are summarized in Tables~\ref{tab:optimal_sources_lmentry}, \ref{tab:optimal_sources_bbh}. The gradual method surfaced as the dominant source of optimal paraphrases across both benchmarks, particularly pronounced in the \lmentry{} benchmark.
However, a closer look at individual models revealed a pattern of preference for different generation methods.

% Some models consistently excel in specific metrics.
\remove{
\begin{table}[!htbp]
\resizebox{\columnwidth}{!}{%
\begin{tabular}{l|cccc}
\hline
\textbf{}                & \textbf{average}    & \textbf{maximum}    & \textbf{saturation} & \textbf{combined}   \\ \hline
\textbf{t0\_3b}          & 7.40                & \underline{12.2}       & 5.9                 & 7.9                 \\
\textbf{t0++}            & 6.32                & 8.00                & 5.08                & 6.20                \\
\textbf{falcon-7b}       & 7.48                & 7.76                & 6.68                & 7.32                \\
\textbf{mpt-7b}          & 9.52                & 10.04               & 8.80                & 9.72                \\
\textbf{alpaca-7b}       & \underline{13.9}       & 7.90                & \underline{13.6}       & \underline{13.2}       \\
\textbf{alpaca-13b}      & 7.32                & 5.80                & 7.32                & 7.40                \\
\textbf{flan-t5-small}   & 6.20                & 9.60                & 7.90                & 5.90                \\
\textbf{flan-t5-base}    & 8.00                & 10.50               & 6.50                & 8.20                \\
\textbf{flan-t5-large}   & 4.10                & 8.50                & 4.80                & 4.50                \\
\textbf{flan-t5-xl}      & 2.72                & 3.16                & 4.68                & 3.08                \\
\textbf{flan-t5-xxl}     & {\underline{ \textbf{1.40}}} & {\underline{\textbf{2.36}}} & {\underline{\textbf{3.40}}} & {\underline{\textbf{1.48}}} \\
\textbf{airoboros-13b}   & 7.24                & 7.48                & 7.28                & 7.60                \\
\textbf{nous-hermes-13b} & 7.68                & 5.76                & 8.76                & 7.56                \\
\textbf{ultralm-13b}     & 10.04               & 7.88                & 8.96                & 9.48                \\
\textbf{vicuna-13b}      & 6.56                & 3.36                & 9.04                & 6.52                \\
\textbf{minotaur-15b}    & 11.88               & 9.88                & 8.52                & 11.76               \\ \hline
\end{tabular}%
}
\caption{\label{tab:model_rankings_avg_new} 
\mnote{new average rank per metric table}
Bold numbers indicate the best averaged rank per metric, while underlined numbers indicate the worst averaged rank per metric.
}
\end{table}
}

\begin{table}[]
\resizebox{\columnwidth}{!}{%
\begin{tabular}{l|cccc}
\hline
\textbf{}                & \textbf{average}    & \textbf{maximum}    & \textbf{saturation} & \textbf{combined}   \\ \hline
\textbf{t0\_3b}          & 7.40                & \underline{12.20}       & 5.90                 & 7.90                 \\
\textbf{t0++}            & 4.80                & 8.80                & 4.20                & 4.63                \\
\textbf{falcon-7b}       & 9.40                & 8.00                & 9.70                & 8.27                \\
\textbf{mpt-7b}          & 10.30               & 11.10               & 10.00               & 10.00               \\
\textbf{alpaca-7b}       & \underline{13.90}       & 7.90                & 13.60       & 13.20      \\
\textbf{alpaca-13b}      & 11.50                & 6.60                & 12.40               & 10.72               \\
\textbf{flan-t5-small}   & 6.20                & 9.60                & 7.90                & 5.90                \\
\textbf{flan-t5-base}    & 8.00                & 10.50               & 6.50                & 8.20                \\
\textbf{flan-t5-large}   & 4.10                & 8.50                & 4.80                & 4.50                \\
\textbf{flan-t5-xl}      & 2.80                & 4.20                & 5.80                & 3.72                \\
\textbf{flan-t5-xxl}     & {{\textbf{1.40}}} & {{\textbf{3.10}}} & {{\textbf{3.70}}} & {{\textbf{1.72}}} \\
\textbf{airoboros-13b}   & 9.50                & 10.20               & 9.50                & 10.36               \\
\textbf{nous-hermes-13b} & 8.90                & 6.30                & 9.70                & 8.73                \\
\textbf{ultralm-13b}     & 12.30               & 9.80                & 9.30                & 11.09               \\
\textbf{vicuna-13b}      & 11.80               & 3.70                & \underline{14.70}               & 10.63               \\
\textbf{minotaur-15b}    & 13.70               & 10.20               & 8.30                & \underline{13.63}               \\ \hline
\end{tabular}%
}\caption{\label{tab:model_rankings_avg_new_lmentry} Average model ranks for each metric across all tasks in \lmentry{}. 
Bold numbers indicate the best averaged rank per metric, while underlined numbers indicate the worst averaged rank per metric.
}
\end{table}

\begin{table}[]
\resizebox{\columnwidth}{!}{%
\begin{tabular}{l|cccc}
\hline
\textbf{}                & \textbf{average}    & \textbf{maximum}    & \textbf{saturation} & \textbf{combined}   \\ \hline
\textbf{t0++}            & 7.33                & 7.47                & 5.67                & 7.33                \\
\textbf{falcon-7b}       & 6.20                & 7.60                & 4.67                & 6.47                \\
\textbf{mpt-7b}          & 9.00                & 9.33                & 8.00                & 9.53                \\
\textbf{alpaca-13b}      & 4.53                & 5.27                & 3.93                & 4.67                \\
\textbf{flan-t5-xl}      & 2.67                & 2.47                & 3.93                & 2.67                \\
\textbf{flan-t5-xxl}     & {{\textbf{1.40}}} & {{\textbf{1.87}}} & {{\textbf{3.20}}} & {{\textbf{1.33}}} \\
\textbf{airoboros-13b}   & 5.73                & 5.67                & 5.80                & 5.67                \\
\textbf{nous-hermes-13b} & 6.87                & 5.40                & 8.13                & 6.67                \\
\textbf{ultralm-13b}     & 8.53                & 6.60                & \underline{8.73}                & 8.20                \\
\textbf{vicuna-13b}      & 3.07                & 3.13                & 5.27                & 3.13                \\
\textbf{minotaur-15b}    & \underline{10.67}               & \underline{9.67}                & 8.67                & \underline{10.33 }              \\ \hline
\end{tabular}%
}\caption{\label{tab:model_rankings_avg_new_bbh} 
Average model ranks for each metric across all tasks in \bbh{}.
Bold numbers indicate the best averaged rank per metric, while underlined numbers indicate the worst averaged rank per metric.
}
\end{table}

% Models show preferences for specific paraphrase generation techniques:
% Please add the following required packages to your document preamble:
% \usepackage{graphicx}
% \usepackage[table,xcdraw]{xcolor}
% Beamer presentation requires \usepackage{colortbl} instead of \usepackage[table,xcdraw]{xcolor}
\begin{table}[!htbp]
\resizebox{\columnwidth}{!}{%
\begin{tabular}{lcccc}
\toprule
\textbf{model}                                  & \textbf{default}                     & \textbf{rephrase}                     & \textbf{cot}                          & \textbf{gradual}                      \\ \hline
\textbf{t0\_3b   (*)}                           & 0.00                                 & 11.76                                 & \textbf{58.82}                        & 29.41                                 \\
\textbf{t0++ (*)}                               & 0.00                                 & 15.00                                 & \textbf{45.00}                        & 40.00                                 \\
\textbf{falcon-7b}                              & 9.09                                 & 9.09                                  & 36.36                                 & \textbf{45.45}                        \\
\textbf{mpt-7b}                                 & 0.00                                 & 23.53                                 & \textbf{47.06}                        & 29.41                                 \\
\textbf{alpaca-7b (**)}                         & 8.33                                 & 0.00                                  & 0.00                                  & \textbf{91.67}                        \\
\textbf{alpaca-13b (**)}                        & 0.00                                 & 0.00                                  & 8.33                                  & \textbf{91.67}                        \\
\textbf{flan-t5-base (*)}                       & 0.00                                 & 7.14                                  & \textbf{64.29}                        & 28.57                                 \\
\textbf{flan-t5-small (*)}                      & 0.00                                 & 0.00                                  & \textbf{58.33}                        & 41.67                                 \\
\textbf{flan-t5-large (*)}                      & 0.00                                 & \textbf{40.00}                        & \textbf{40.00}                        & 20.00                                 \\
\textbf{flan-t5-xl (*)}                         & 0.00                                 & 7.69                                  & 30.77                                 & \textbf{61.54}                        \\
\textbf{flan-t5-xxl (*)}                        & 0.00                                 & 13.04                                 & \textbf{69.57}                        & 17.39                                 \\
\textbf{airoboros-13b (**)}                     & 0.00                                 & 35.71                                 & 14.29                                 & \textbf{50.00}                        \\
\textbf{nous-hermes-13b   (**)}                 & 0.00                                 & 0.00                                  & 33.33                                 & \textbf{66.67}                        \\
\textbf{ultralm-13b (**)}                       & 0.00                                 & 6.67                                  & \textbf{66.67}                        & 26.67                                 \\
\textbf{vicuna-13b (**)}                        & 10.00                                & 10.00                                 & 0.00                                  & \textbf{80.00}                        \\
\textbf{minotaur-15b}                           & 0.00                                 & 14.29                                 & 28.57                                 & \textbf{57.14}                        \\ \hline
{\color[HTML]{4472C4} \textbf{all models}}      & {\color[HTML]{0070C0} \textbf{1.33}} & {\color[HTML]{0070C0} \textbf{12.39}} & {\color[HTML]{0070C0} \textbf{40.71}} & {\color[HTML]{0070C0} \textbf{45.58}} \\
{\color[HTML]{00B050} \textbf{all paraphrases}} & {\color[HTML]{00B050} \textbf{1.24}} & {\color[HTML]{00B050} \textbf{18.98}} & {\color[HTML]{00B050} \textbf{52.94}} & {\color[HTML]{00B050} \textbf{26.84}} \\ \bottomrule
\end{tabular}%
}
\caption{Distribution of optimal paraphrase sources per model for \lmentry{}. Rows represent models, with T5-based models marked by an asterisk (*) and \llama{}-based models by two asterisks (**). Columns indicate paraphrase generation methods. Percentages in each cell show the rate of optimal paraphrases from each method, with bold numbers identifying the leading source for each model. The `All Models' row aggregates percentages across all models, while the `All Paraphrases' row displays the overall distribution of generation methods across all paraphrases.}
\label{tab:optimal_sources_lmentry}
\end{table}
% Please add the following required packages to your document preamble:
% \usepackage{graphicx}
% \usepackage[table,xcdraw]{xcolor}
% Beamer presentation requires \usepackage{colortbl} instead of \usepackage[table,xcdraw]{xcolor}
\begin{table}[!htbp]
\resizebox{\columnwidth}{!}{%
\begin{tabular}{lllll}
\toprule
\textbf{model}                                  & \textbf{default}                     & \textbf{rephrase}                     & \textbf{cot}                          & \textbf{gradual}                      \\ \hline
\textbf{falcon-7b}                              & 0.00                                 & 27.27                                 & 18.18                                 & \textbf{54.55}                        \\
\textbf{mpt-7b}                                 & 0.00                                 & 40.00                                 & 16.00                                 & \textbf{44.00}                        \\
\textbf{flan-t5-xl}                             & 2.38                                 & 23.81                                 & 26.19                                 & \textbf{47.62}                        \\
\textbf{flan-t5-xxl}                            & 4.35                                 & 17.39                                 & 26.09                                 & \textbf{52.17}                        \\
\textbf{t0++}                                   & 0.00                                 & \textbf{50.00}                        & 40.00                                 & 10.00                                 \\
\textbf{alpaca-13b}                             & 0.00                                 & 11.11                                 & \textbf{44.44}                        & \textbf{44.44}                        \\
\textbf{airoboros-13b}                          & 0.00                                 & \textbf{50.00}                        & 16.67                                 & 33.33                                 \\
\textbf{nous-hermes-13b}                        & 0.00                                 & 12.50                                 & 16.67                                 & \textbf{70.83}                        \\
\textbf{ultralm-13b}                            & 0.00                                 & 29.17                                 & 25.00                                 & \textbf{45.83}                        \\
\textbf{vicuna-13b}                             & 0.00                                 & \textbf{38.10}                        & 28.57                                 & 33.33                                 \\
\textbf{minotaur-15b}                           & 0.00                                 & 9.09                                  & 0.00                                  & \textbf{90.91}                        \\ \hline
{\color[HTML]{4472C4} \textbf{all tasks}}       & {\color[HTML]{4472C4} \textbf{0.73}} & {\color[HTML]{4472C4} \textbf{27.37}} & {\color[HTML]{4472C4} \textbf{23.72}} & {\color[HTML]{4472C4} \textbf{48.18}} \\
{\color[HTML]{00B050} \textbf{all paraphrases}} & {\color[HTML]{00B050} \textbf{0.57}} & {\color[HTML]{00B050} \textbf{28.07}} & {\color[HTML]{00B050} \textbf{29.64}} & {\color[HTML]{00B050} \textbf{41.72}} \\ \bottomrule
\end{tabular}%
}
\caption{Distribution of optimal paraphrase sources per model for \bbh{}. Rows represent models and columns indicate paraphrase generation methods. Percentages in each cell show the rate of optimal paraphrases from each method, with bold numbers identifying the leading source for each model. The `All Models' row aggregates percentages across all models, while the `All Paraphrases' row displays the overall distribution of generation methods across all paraphrases.}
\label{tab:optimal_sources_bbh}
\end{table}
}
% LLaMA models lag in saturation compared to T5 models in LMentry:
% \begin{figure}[p]
% \includegraphics[width=\linewidth]{figures/notable_failures_count3.png}
% \caption{\label{fig:notable_failures_lmentry}
% Number of notable failures (accuracy below 5\%) in \llama{} models (blue) vs. T5 models (purple) on \lmentry{} Tasks.
% }\end{figure}

\remove{
\subsection{Small Scale Evaluation - OpenAI}
This subsection contains all the tables referenced in Section~\ref{sec:openai_evaluation}. Table~\ref{tab:openai_avg_repetitions} and Table~\ref{tab:openai_max_heuristic} are related to our naive heuristics for estimating average and maximum performance, respectively. Table~\ref{tab:openai_avg_repetitions} presents the average number of repetitions needed for our heuristic to estimate the average performance, ensuring less than a 1-point accuracy discrepancy from the actual average for each open-source model across all tasks in the \lmentry{} benchmark. Table~\ref{tab:openai_max_heuristic} compiles results from our greedy heuristic that searches for the optimal paraphrases for each open-source model on each \lmentry{} task.

Table~\ref{tab:openai_avg_deafult} and Table~\ref{tab:openai_max_default} aggregate the average and maximum performances for each model and task using only the original instruction templates. Similarly, Table~\ref{tab:openai_avg_all} and Table~\ref{tab:openai_max_all} present the approximated average and maximum performances, computed with our heuristics, for each model and task using all paraphrased templates.

Table~\ref{tab:openai_mecnemar} contains the McNemar test p-values we used to assess the statistical significance of the differences in maximum performance between the original best prompt and the estimated optimal prompt. 

% Finally, Table~\ref{tab:openai_edit_distance} shows representative examples of instruction template pairs with very minor differences but notable variations in performance.

% Please add the following required packages to your document preamble:
% \usepackage{graphicx}
\begin{table*}[!htbp]
\begin{adjustwidth}{-1cm}{-1cm}
\resizebox{1.1\textwidth}{!}{%
\begin{tabular}{l|cccccccccccccccc}
\toprule
\textbf{task}                      & \textbf{t0\_3b} & \textbf{t0++} & \textbf{fal7b} & \textbf{mpt7b} & \textbf{alp7b} & \textbf{alp13b} & \textbf{ft5small} & \textbf{ft5base} & \textbf{ft5large} & \textbf{ft5xl} & \textbf{ft5xxl} & \textbf{airoboros} & \textbf{noushermes} & \textbf{ultralm} & \textbf{vicuna} & \textbf{minotaur} \\ \hline
\textbf{all words from   category} & 4.9             & 2.2           & 11.3               & 4.2             & 3.1                & 2.9                 & 5.6                    & 4.3                   & 2.4                    & 6.6                 & 3.1                  & 6.6                    & 8.7                      & 3.2                  & 3.8                 & 7.5                   \\
\textbf{any words from   category} & 3.4             & 1.5           & 11.2               & 4.1             & 3.8                & 2.9                 & 11                     & 7.3                   & 6.7                    & 2                   & 1.7                  & 5.8                    & 3.2                      & 6                    & 2.6                 & 2.1                   \\
\textbf{ends with word}            & 3.3             & 4.3           & 2.2                & 2.4             & 1.9                & 10.7                & 3.3                    & 6.2                   & 5.7                    & 5.9                 & 6.1                  & 2.8                    & 3.5                      & 2                    & 3.7                 & 2.5                   \\
\textbf{first   alphabetically}    & 10.3            & 3.2           & 7.2                & 6.1             & 2.6                & 6.4                 & 10.3                   & 3.2                   & 5.1                    & 3.9                 & 4                    & 5.3                    & 8.2                      & 11.4                 & 5.7                 & 7.8                   \\
\textbf{homophones}                & 7.2             & 5.7           & 8.3                & 10.3            & 2.4                & 4.2                 & 10.5                   & 4.5                   & 3.5                    & 3.7                 & 9.7                  & 5.8                    & 10.8                     & 2.1                  & 3.7                 & 1.2                   \\
\textbf{less letters}              & 3.3             & 9.5           & 5.3                & 3.8             & 4.2                & 5.5                 & 5.9                    & 4.6                   & 4.5                    & 5.1                 & 3.5                  & 4.2                    & 3.5                      & 7.1                  & 10.2                & 6.3                   \\
\textbf{more letters}              & 4.3             & 4.2           & 6.5                & 6               & 5.8                & 10.4                & 3.3                    & 4.2                   & 4.2                    & 4.9                 & 7.6                  & 5.4                    & 9.3                      & 6                    & 7.9                 & 6.8                   \\
\textbf{rhyming word}              & 10.9            & 2.5           & 4.1                & 5.2             & 2.6                & 12.8                & 6.6                    & 3.8                   & 6.7                    & 5.1                 & 5.6                  & 3.3                    & 3.8                      & 1.8                  & 7.3                 & 1.2                   \\
\textbf{word before}               & 5.9             & 2.8           & 1.3                & 3.2             & 6.6                & 3.5                 & 6                      & 4.4                   & 4.5                    & 8.8                 & 4.9                  & 4.5                    & 3.3                      & 1.1                  & 5.1                 & 2                     \\
\textbf{word not   containing}     & 4.2             & 12.4          & 8.6                & 11.8            & 9.4                & 6.3                 & 4.4                    & 10                    & 21.9                   & 14.2                & 5.8                  & 10.1                   & 5.8                      & 6.3                  & 5                   & 12.3 \\ \bottomrule                
\end{tabular}%
}
\caption{The average number of average heuristic repetitions required to achieve less than a 1 accuracy point discrepancy from the actual average performance for each task and open-source model. Maximal value: 21.9. All values average: 5.62 (std: 3.12).}
\label{tab:openai_avg_repetitions}
\end{adjustwidth}
\end{table*}
%Generate Result (click "Generate" to refresh) Copy to clipboard
% Please add the following required packages to your document preamble:
% \usepackage{graphicx}
\begin{table*}[!htbp]
\begin{adjustwidth}{-1cm}{-1cm}
\resizebox{1.1\textwidth}{!}{%
\begin{tabular}{l|cccccccccccccccc}
\toprule
\textbf{task}                      & \textbf{t0\_3b} & \textbf{t0++} & \textbf{fal7b} & \textbf{mpt7b} & \textbf{alp7b} & \textbf{alp13b} & \textbf{ft5small} & \textbf{ft5base} & \textbf{ft5large} & \textbf{ft5xl} & \textbf{ft5xxl} & \textbf{airoboros} & \textbf{noushermes} & \textbf{ultralm} & \textbf{vicuna} & \textbf{minotaur} \\ \hline
\textbf{all words from   category} & \checkmark{}              & \checkmark{}            & 0.01           & \checkmark{}             & \checkmark{}             & \checkmark{}              & 0.03              & \checkmark{}               & 0.02              & \checkmark{}             & \checkmark{}              & \checkmark{}                 & 0.02                & \checkmark{}               & \checkmark{}              & \checkmark{}                \\
\textbf{any words from   category} & \checkmark{}              & \checkmark{}            & \checkmark{}             & \checkmark{}             & \checkmark{}             & \checkmark{}              & \checkmark{}                & \checkmark{}               & \checkmark{}                & \checkmark{}             & \checkmark{}              & \checkmark{}                 & 0.06                & \checkmark{}               & \checkmark{}              & \checkmark{}                \\
\textbf{ends with word}            & \checkmark{}              & \checkmark{}            & \checkmark{}             & \checkmark{}             & \checkmark{}             & \checkmark{}              & \checkmark{}                & \checkmark{}               & \checkmark{}                & \checkmark{}             & \checkmark{}              & \checkmark{}                 & \checkmark{}                  & \checkmark{}               & \checkmark{}              & 0.03              \\
\textbf{first   alphabetically}    & \checkmark{}              & \checkmark{}            & \checkmark{}             & \checkmark{}             & \checkmark{}             & \checkmark{}              & 0.01              & \checkmark{}               & 0.03              & 0.03           & \checkmark{}              & \checkmark{}                 & \checkmark{}                  & \checkmark{}               & \checkmark{}              & \checkmark{}                \\
\textbf{homophones}                & \checkmark{}              & \checkmark{}            & \checkmark{}             & \checkmark{}             & \checkmark{}             & \checkmark{}              & \checkmark{}                & \checkmark{}               & 0.04              & \checkmark{}             & \checkmark{}              & \checkmark{}                 & \checkmark{}                  & \checkmark{}               & \checkmark{}              & 0.01              \\
\textbf{less letters}              & \checkmark{}              & 0.02          & 0.01           & \checkmark{}             & \checkmark{}             & \checkmark{}              & 0.02              & \checkmark{}               & 0.03              & \checkmark{}             & 0.02            & \checkmark{}                 & \checkmark{}                  & \checkmark{}               & \checkmark{}              & \checkmark{}                \\
\textbf{more letters}              & 0.01            & 0.01          & \checkmark{}             & 0.03           & \checkmark{}             & \checkmark{}              & \checkmark{}                & \checkmark{}               & \checkmark{}                & 0.01           & \checkmark{}              & \checkmark{}                 & \checkmark{}                  & 0.01             & \checkmark{}              & \checkmark{}                \\
\textbf{rhyming word}              & \checkmark{}              & 0.01          & \checkmark{}             & \checkmark{}             & \checkmark{}             & \checkmark{}              & 0.02              & 0.03             & 0.01              & 0.01           & \checkmark{}              & \checkmark{}                 & \checkmark{}                  & 0.01             & \checkmark{}              & \checkmark{}                \\
\textbf{word before}               & \checkmark{}              & \checkmark{}            & \checkmark{}             & \checkmark{}             & 0.01           & \checkmark{}              & \checkmark{}                & \checkmark{}               & \checkmark{}                & \checkmark{}             & 0.06            & \checkmark{}                 & \checkmark{}                  & \checkmark{}               & 0.01            & \checkmark{}                \\
\textbf{word not   containing}     & \checkmark{}              & \checkmark{}            & \checkmark{}             & \checkmark{}             & \checkmark{}             & \checkmark{}              & \checkmark{}                & \checkmark{}               & \checkmark{}                & \checkmark{}             & \checkmark{}              & \checkmark{}                 & \checkmark{}                  & \checkmark{}               & \checkmark{}              & \checkmark{}    \\ \hline           
\end{tabular}%
}
\caption{Results of the greedy optimal paraphrase search for each task and open-source model. An optimal prompt was recovered in 130 out of 160 cases. In the remaining cases, the average discrepancy in performance between the chosen and actual optimal paraphrases was 2.1 accuracy points, with a standard deviation of 1.4.}
\label{tab:openai_max_heuristic}
\end{adjustwidth}
\end{table*}
% Please add the following required packages to your document preamble:
% \usepackage{graphicx}
\begin{table}[!htbp]
\resizebox{\columnwidth}{!}{%
\begin{tabular}{lcccc} \toprule
                                   & \multicolumn{1}{c}{\textbf{davinci}} & \multicolumn{1}{c}{\textbf{td002}} & \multicolumn{1}{c}{\textbf{td003}} & \multicolumn{1}{c}{\textbf{cgpt}} \\ \hline
\textbf{all words from   category} & 0.56                                 & 0.72                               & 0.84                               & 0.60                              \\
\textbf{any words from   category} & 0.55                                 & 0.63                               & 0.65                               & 0.86                              \\
\textbf{ends with word}            & 0.10                                 & 0.30                               & 0.58                               & 0.60                              \\
\textbf{first   alphabetically}    & 0.46                                 & 0.48                               & 0.71                               & 0.98                              \\
\textbf{homophones}                & 0.48                                 & 0.19                               & 0.38                               & 0.49                              \\
\textbf{less letters}              & 0.41                                 & 0.67                               & 0.79                               & 0.88                              \\
\textbf{more letters}              & 0.47                                 & 0.68                               & 0.82                               & 0.87                              \\
\textbf{rhyming word}              & 0.19                                 & 0.29                               & 0.57                               & 0.69                              \\
\textbf{word before}               & 0.12                                 & 0.13                               & 0.27                               & 0.40                              \\
\textbf{word not   containing}     & 0.03                                 & 0.85                               & 0.97                               & 0.90      \\ \bottomrule                       
\end{tabular}%
}
\caption{
 Average performances for OpenAI models across all \lmentry{} tasks, computed using only the original prompts.
 }
\label{tab:openai_avg_deafult}
\end{table}
% Please add the following required packages to your document preamble:
% \usepackage{graphicx}
\begin{table}[!htbp]
\resizebox{\columnwidth}{!}{%
\begin{tabular}{lcccc} \toprule
                                   & \multicolumn{1}{c}{\textbf{davinci}} & \multicolumn{1}{c}{\textbf{td002}} & \multicolumn{1}{c}{\textbf{td003}} & \multicolumn{1}{c}{\textbf{cgpt}} \\ \hline
\textbf{all words from   category} & 0.15                                 & 0.61                               & 0.79                               & 0.62                              \\
\textbf{any words from   category} & 0.16                                 & 0.62                               & 0.59                               & 0.82                              \\
\textbf{ends with word}            & 0.11                                 & 0.24                               & 0.42                               & 0.54                              \\
\textbf{first   alphabetically}    & 0.12                                 & 0.27                               & 0.35                               & 0.45                              \\
\textbf{homophones}                & 0.12                                 & 0.57                               & 0.60                               & 0.71                              \\
\textbf{less letters}              & 0.17                                 & 0.51                               & 0.58                               & 0.58                              \\
\textbf{more letters}              & 0.16                                 & 0.49                               & 0.51                               & 0.50                              \\
\textbf{rhyming word}              & 0.14                                 & 0.39                               & 0.41                               & 0.76                              \\
\textbf{word before}               & 0.04                                 & 0.16                               & 0.51                               & 0.47                              \\
\textbf{word not   containing}     & 0.06                                 & 0.57                               & 0.84                               & 0.81      \\ \bottomrule                       
\end{tabular}%
}
\caption{Estimated average performances for OpenAI models across all \lmentry{} tasks, approximated using all prompt paraphrases.}
\label{tab:openai_avg_all}
\end{table}
% Please add the following required packages to your document preamble:
% \usepackage{graphicx}
\begin{table}[!htbp]
\resizebox{\columnwidth}{!}{%
\begin{tabular}{lcccc} \toprule
                                   & \multicolumn{1}{c}{\textbf{davinci}} & \multicolumn{1}{c}{\textbf{td002}} & \multicolumn{1}{c}{\textbf{td003}} & \multicolumn{1}{c}{\textbf{cgpt}} \\ \hline
\textbf{all words from   category} & 0.64                                 & 0.80                               & 0.85                               & 0.68                              \\
\textbf{any words from   category} & 0.66                                 & 0.82                               & 0.88                               & 0.97                              \\
\textbf{ends with word}            & 0.15                                 & 0.35                               & 0.61                               & 0.62                              \\
\textbf{first   alphabetically}    & 0.50                                 & 0.56                               & 0.90                               & 0.98                              \\
\textbf{homophones}                & 0.59                                 & 0.25                               & 0.41                               & 0.79                              \\
\textbf{less letters}              & 0.48                                 & 0.70                               & 0.86                               & 0.92                              \\
\textbf{more letters}              & 0.54                                 & 0.80                               & 0.89                               & 0.90                              \\
\textbf{rhyming word}              & 0.32                                 & 0.45                               & 0.65                               & 0.96                              \\
\textbf{word before}               & 0.17                                 & 0.21                               & 0.34                               & 0.66                              \\
\textbf{word not   containing}     & 0.04                                 & 0.92                               & 1.00                               & 0.96      \\ \bottomrule                       
\end{tabular}%
}
\caption{Max performances for OpenAI models across all \lmentry{} tasks, computed using only the original prompts.}
\label{tab:openai_max_default}
\end{table}
% Please add the following required packages to your document preamble:
% \usepackage{graphicx}
\begin{table}[!htbp]
\resizebox{\columnwidth}{!}{%
\begin{tabular}{lcccc} \toprule
                                   & \multicolumn{1}{c}{\textbf{davinci}} & \multicolumn{1}{c}{\textbf{td002}} & \multicolumn{1}{c}{\textbf{td003}} & \multicolumn{1}{c}{\textbf{cgpt}} \\ \hline
\textbf{all words from   category} & 0.64                                 & 0.94                               & 0.99                               & 0.97                              \\
\textbf{any words from   category} & 0.66                                 & 0.95                               & 0.99                               & 1.00                              \\
\textbf{ends with word}            & 0.88                                 & 0.52                               & 0.67                               & 0.72                              \\
\textbf{first   alphabetically}    & 0.55                                 & 0.95                               & 0.97                               & 1.00                              \\
\textbf{homophones}                & 0.63                                 & 0.99                               & 0.95                               & 0.99                              \\
\textbf{less letters}              & 0.61                                 & 0.95                               & 0.95                               & 1.00                              \\
\textbf{more letters}              & 0.71                                 & 0.93                               & 0.97                               & 1.00                              \\
\textbf{rhyming word}              & 0.67                                 & 0.93                               & 0.95                               & 0.99                              \\
\textbf{word before}               & 0.26                                 & 0.51                               & 0.82                               & 0.95                              \\
\textbf{word not   containing}     & 0.65                                 & 1.00                               & 1.00                               & 1.00   \\ \bottomrule                          
\end{tabular}%
}
\caption{Estimated max performances for OpenAI models across all \lmentry{} tasks, approximated using all prompt paraphrases.}
\label{tab:openai_max_all}
\end{table}

% Please add the following required packages to your document preamble:
% \usepackage{graphicx}
% \usepackage[normalem]{ulem}
% \useunder\underline{ine}\underline{}{}
\begin{table}[!htbp]
\begin{adjustwidth}{-0.5cm}{0cm}
\resizebox{1.05\columnwidth}{!}{%
\begin{tabular}{lcccc} \toprule
\textbf{task}                      & \textbf{davinci}        & \textbf{td002}          & \textbf{td003}          & \textbf{cgpt}           \\ \hline
\textbf{all words from   category} & 1                       & \underline{{.0009}} & \underline{{.0002}} & \underline{{7.2E-08}} \\
\textbf{any words from category} & 1                       & \underline{{.0008}} & \underline{{.0009}} & .0832                \\
\textbf{ends with word}            & \underline{{8.8E-17}} & \underline{{.0195}} & .3034                & .0955                \\
\textbf{first   alphabetically}    & .4922                & \underline{{6.1E-09}} & \underline{{.0196}} & .1572                \\
\textbf{homophones}                & .5371               & \underline{{7.8E-18}} & \underline{{5.3E-13}} & \underline{{7.7E-06}} \\
\textbf{less letters}              & .0633                & \underline{{3.4E-06}} & \underline{{.0009}} & \underline{{.0047}} \\
\textbf{more letters}              & \underline{{.0131}} & \underline{{.0046}} & \underline{{.0209}} & \underline{{.0016}} \\
\textbf{rhyming word}              & \underline{{5.7E-07}} & \underline{{1.4E-10}} & \underline{{4.3E-08}} & .0833                \\
\textbf{word before}               & .10560                & \underline{{1.1E-06}} & \underline{{1.1E-11}} & \underline{{1.9E-06}} \\
\textbf{word not containing}       & \underline{{6.3E-05}} & .1573                & 1                       & .3173 \\ \bottomrule               
\end{tabular}
}\caption{
The results for the McNemar test we ran to assess the statistical significance of the differences in maximum performance between the original best prompt and the prompt estimated to be optimal across all paraphrases for each task in the \lmentry{} benchmark. Significant max differences (p-value<0.05) are highlighted. 
}
\label{tab:openai_mecnemar}
\end{adjustwidth}
\end{table}
}
